# Supplementary material for: A-D-E diagrams, Hodge--Tate hyperplane sections and semisimple quantum cohomology
Source: arXiv:2509.01101 source file (2026-09-27)
Supplement: Supplementary file 1 [file appendix-preamble.tex]

\usepackage{colonequals}

\newtheorem{theorem}[thm]{Theorem}
\newtheorem{proposition}[thm]{Proposition}

\makeatletter
% Redefine \paragraph to match article.cls
\renewcommand\paragraph{%
  \@startsection{paragraph}{4}%
    {\z@}% indent
    {3.25ex \@plus 1ex \@minus .2ex}% beforeskip
    {-1em}% afterskip (negative = run-in heading)
    {\normalfont\normalsize\bfseries}%
}
\makeatletter

\newcommand\kronecker[3]{\ensuremath{\mathrm{M}_{(#2,#3)}^{#1}}}
\newcommand\poincare[3]{\ensuremath{\mathrm{P}_{(#2,#3)}^{#1}}}
\newcommand\qbinom{\genfrac{[}{]}{0pt}{}}

\newcommand\ee{\ensuremath{\mathrm{e}}}
\newcommand\ii{\ensuremath{\mathrm{i}}}

\DeclareMathOperator\Gr{Gr}
\DeclareMathOperator\QH{QH}
